# Supplementary material for: The Effects of Invertibility on the Representational Complexity of Encoders in Variational Autoencoders
Source: arXiv:2107.04652 source file (2021-07-09)
Supplement: Supplementary file 1 [file main_together.tex]

\subsection{Initialization} \label{sS-initialization}

In this section, we prove a guarantee on the distance of a convenient initialization for $z_0$ for Lemma \ref{lem-MainSampling}. \footnote{Note, the initialization isn't merely taking $z_0 = z_{init}$ -- we will add a bit of noise to $z_{init}$. This is the reason behind the choice of notation for $z_{init}$.} 
To draw a sample from the initial distribution for $z_0$, we set it to $z_0 := z_{init} + N$ where $N$ is sampled from a uniform distribution given by $N \sim \mbox{Unif} \left( B \right)$, where $B := \{ z : \|z\| \leq \frac{1}{4} rad(\D) \}$. Let us denote by $\tilde{P}_0$ the distribution of this $z_0$.

% the main sampling lemma using Lemma \ref{lem-restricted}: where the $\alpha$ term is from lemma \ref{lem-concentrationD}, and the $\mainpc$ term is from lemma \ref{lem-mainpc}.

% ---
% We need one more technical helper lemma before proceeding to the proof. 
% \begin{lemma} \label{lem-FtimesRECF_integral}
%     Let $I = \int_{x \in \Q } e^{f(x)} dx$. Let $J = \int_{x \in \Q } e^{-f(x)} dx$. Then we have
%     \[ IJ \leq e^{\sup_{x \in \Q} f(x) - \inf_{x \in \Q} f(x) } \cdot \mbox{vol}(\Q)^2 \]
%     Where $\mbox{vol}(\Q)$ denotes the volume of $\Q$.
% \end{lemma}
% \begin{proof}
%     Proof is immediate using the fact that 
%     \[ e^{f(x)} \leq e^{ \sup_{x \in \Q} f(x)} \qquad x \in \Q \]
%     \[ e^{-f(x)} \leq e^{ - \inf_{x \in \Q} f(x)} \qquad x \in \Q \]
% \end{proof}
% ---

% --- % --- % --- % --- % --- % --- % --- % --- % --- % --- % --- % --- % --- % --- % --- % --- % --- % --- % --- 
To integrate this with Lemma \ref{lem-MainSampling}, we will show how far this initial distribution is from the target stationary distribution. 

%We first create an initialization scheme for the langevin chain ($z_0$) using the output of the Gradient Descent ($z_{init}$) such that $\chi^2 \left( \tP_0, \tP \right)$ is bounded.
%\Dnote{Add footnote if required: The scheme is <blah> which we will use in theorem \ref{thm-main}. Lemma 3 should have this scheme in the lemma statement.}
\begin{lemma}[Bounding initialization distance for Langevin diffusion] \label{lem-chi2bound}
    %Using $z_{init}$ such that $\| z_{init} - \hz \| \leq \frac{1}{4} rad(\D)$, %we can create a (random) point $z_0$ satisfying $\| z_0 - \hz\| \leq \frac{1}{2} rad(\D)$ such that its distribution $\tP_0$ satisfies
    The distribution $\tilde{P}_0$ for $z_0$ specified above satisfies
    \[ \log \sqrt{ \chi^2 \left( \tP_0, \tP \right) } \leq \O \left( d \cdot \log \frac{d}{\epsilon} \right) \]
    with probability $1 - \exp(-\O(d))$ over $x$ sampled from the generator.
\end{lemma}
\begin{proof}
    %We will set $z_0 := z_{init} + N$ where $N$ is the noise term, following the Uniform distribution given by $N \sim \mbox{Unif} \left( B \right)$, where $B$ is the set defined as 
    %\[ B := \{ z : \|z\| \leq \frac{1}{4} rad(\D) \}\]
    %Note that $z_{init}$ is a deterministic point. So the only randomness in $z_0$ comes from the noise term.
    %Clearly the required condition on $z_0$ holds true because:
    
    %First, note that 
    %\[ \| z_0 - \hz \| \leq \| z_{init} - \hz \| + \|N\| \leq \frac{1}{4} rad(\D) + \frac{1}{4} rad(\D) = \frac{1}{2} rad(\D) \]

    Using the formula for the $\chi^2$-divergence, one can write
    \begin{equation} \label{eq-chi2}
        \chi^2 \left( \tP_0, \tP \right) \leq \int_{z \in \D} \frac{ \tp_0 (z)^2 }{ \tp(z) } dz
    \end{equation}
    where we denote the density of $\tP_0$ with $\tp_0$ and that of $\tP$ with $\tp$. (%We also use the fact that both $\tP_0$ and $\tP$ have no support outside the region $\D$.
    Also, note the expression is well-defined since $\tP$ has support $\D$ and $\tP_0$ has support that is a subset of $\D$.)
    
    Let us denote by $c_d > 0$ the volume of a hypersphere in $d$ dimensions. 
    Since $\tP_0$ is a uniform distribution over a hyper-sphere of radius $\frac{1}{4} rad(\D)$, we have % which is contained inside $\D$, its density \emph{for all} points inside $\D$ is upper bounded by $\frac{1}{c_d}$. Hence, %by the reciprocal of the volume of the hyper-sphere, given as the following (where $c_d > 0$ denotes the constant for the volume of a hyper-sphere in $d$ dimensions)
    \begin{equation} \label{eq-chi2T1}
        \tp_0 (z) \leq \frac{1}{c_d \cdot \left( \frac{1}{4}rad(\D) \right)^d} \qquad z \in \D    
    \end{equation}
    % So we get
    % \[ \chi^2 \left( \tP_0, \tP \right) \leq \frac{4^{2d}}{c_d^2 \cdot rad(\D)^{2d}} \int_{z \in \D} \frac{ 1 }{ \tp(z) } dz \]
    
    On the other hand, 
    \[ \int_{z \in \D} \frac{ 1 }{ \tp(z) } dz = \int_{z \in \D} e^{-L(z)} dz \cdot \int_{z \in \D} \frac{ 1 }{ e^{-L(z)} } dz \]
    From this rewrite, we can conclude
    \begin{equation} \label{eq-chi2T2}
        \int_{z \in \D} \frac{ 1 }{ \tp(z) } dz \leq e^{ - \inf_{z \in \D} L(z)} vol(\D) \cdot e^{\sup_{z \in \D} L(z) }  vol(\D)
    \end{equation}
    Where $vol(\D) = \left( c_d \cdot rad(\D)^d \right)$ using the notation of $c_d$ above.
    
    Plugging in \eqref{eq-chi2T1} and \eqref{eq-chi2T2} in \eqref{eq-chi2}, we get
    \begin{align} \label{eq-chi2Simp}
        \chi^2 \left( \tP_0, \tP \right) &\leq 4^{2d} \cdot e^{\sup_{z \in \D} L(z) - \inf_{z \in \D} L(z) } \nonumber \\ 
        \implies \log \sqrt{\chi^2 \left( \tP_0, \tP \right)} &\leq  d \log 4 + \frac{1}{2} \left( \sup_{z \in \D} L(z) - \inf_{z \in \D} L(z) \right) 
    \end{align}
    
    Using the definition of $L(z)$ from \eqref{eq-Lz} and Assumption \ref{as-M}, we get
    \begin{align} \label{eq-sup}
        \sup_{z \in \D} L(z) \leq \frac{1}{2} \left( \| \hz \| + rad(\D) \right)^2 + \frac{1}{2} \cdot \frac{M^2}{\beta^2} \cdot rad(\D)^2
    \end{align}
  From Assumption \ref{as-bij} we then have: 
  %and lower-bounding the $\inf$ with a larger set, we get
    \begin{align} \label{eq-inf}
        \inf_{z \in \D} L(z) &\geq \inf_{z \in \R^d} \frac{1}{2} \left( \|z\|^2 + \frac{m^2}{\beta^2} \|z - \hz\|^2 \right) \nonumber \\
        &\geq \frac{1}{2} \cdot \frac{m^2}{m^2 + \beta^2} \|\hz\|^2
    \end{align}
    Plugging in \eqref{eq-sup} and \eqref{eq-inf} in \eqref{eq-chi2Simp}, we get that
    \begin{align*}
        \log \sqrt{ \chi^2 \left( \tP_0, \tP \right) } &\leq d \cdot \log 4 + \frac{1}{4} \left( \frac{ \beta^2 }{m^2 + \beta^2} \|\hz\|^2 + 2 \cdot \|\hz\| \cdot rad(\D) + \left( 1 + \frac{M^2}{\beta^2} \right) rad(\D)^2 \right)
    \end{align*}
     Using $\| \hz \| \leq \|x\|/m$ from Lemma \ref{eq-normhz} and $\|x\| \leq \O(\sqrt{d})$ from Lemma \ref{lem-WHPx}, we get
    \begin{align*}
        \log \sqrt{ \chi^2 \left( \tP_0, \tP \right) } &\leq \O(d) +  %\O(\beta^2 d) + 
        \O(\sqrt{d}) \cdot rad(\D) + \left( 1 + \frac{M^2}{\beta^2} \right) rad(\D)^2 
    \end{align*}
    Plugging in $rad(\D)$ from Lemma \ref{lem-concentrationD} and using the bound on $\beta$, we get the desired result.  
    
    %from the same lemma, we get that the last term actually dictates this bound, since $\frac{rad(\D)^2}{\beta^2} = \Theta \left(d \log \frac{d}{\epsilon} \right)$. Hence, we get the desired bound on the divergence.
\end{proof}

% --- % --- % --- % --- % --- % --- % --- % --- % --- % --- % --- % --- % --- % --- % --- % --- % --- % --- % --- 
\subsection{Proof of Lemma \ref{lem-MainSampling}} \label{sS-MainSampling}
We can now put together the proof of Lemma \ref{lem-MainSampling}.
\begin{proof}[Proof of Lemma \ref{lem-MainSampling}]
Using Lemma \ref{lem-restricted} with $\D$ defined as in Lemma \ref{lem-concentrationD},
with $\alpha := \epsilon/4$ in Lemma \ref{lem-concentrationD} and the $\mainpc$ bound from  Lemma \ref{lem-mainpc}, setting 
\[ T = \frac{4}{\pi} rad(\D) \cdot \left( \log \sqrt{\chi^2 \left( \tP_0, \tP \right)} + \log \frac{1}{\epsilon} \right)  \]
we get 
%$T$ such that
\begin{align*}
    \frac{1}{2} \sqrt{\chi^2 \left( \tP_0, \tP \right)} e^{-T / 2 \mainpc} &\leq \frac{\epsilon}{2} \\
 %   \implies T &= 2 \mainpc \cdot \left( \log \sqrt{\chi^2 \left( \tP_0, \tP \right)} + \log \frac{1}{\epsilon} \right) 
\end{align*}
Using $rad(\D) = \O(1 / d)$ from lemma \ref{def-D}, and the bound on the $\chi^2$ term as $\O(d \log d/\epsilon)$ from Lemma \ref{lem-chi2bound}, the result follows.
% The result is a $\mbox{TV}$-guarantee between the langevin chain's distribution $P_T$ and its stationary distribution $P$, which is the same as the true posterior $p(z | x)$ from equation \eqref{eq-Lz} -- as written in the lemma statement.
%Assigning $\epsilon := \epsilon/2$ gives the exact lemma statement.
\end{proof}

% \paragraph{Remark: } We
