# Supplementary material for: The Effects of Invertibility on the Representational Complexity of Encoders in Variational Autoencoders
Source: arXiv:2107.04652 source file (2021-07-09)
Supplement: Supplementary file 2 [file scratch_tv.tex]

\section{Scratch TV distance}

Let us consider two points $z, z'\in \mathcal{D}$. We will show that after $T$ steps of the Langevin chain, the distribution $P_T$ satisfies
\begin{equation}
    d_{\mbox{TV}}(P_T z, P_T z') \leq \frac{\|z-z'\|}{\sqrt{2 \pi T}} + \epsilon/4
\label{eq:tvlang}
\end{equation}
The proof is same as Lemma 4 in \citejournal{bubeck2018sampling}. %we have $ d_{\mbox{TV}}(P_T z, P_T z') \leq \Pr[Z_t \neq Z'_t]$ for any coupling of two random variables $Z_t, Z'_t$ that marginally follow the distribution of the Langevin chain. 
Consider the reflection coupling that reflects the Brownian motion around the separating hyperplane between $Z_t, Z'_t$ until the (random) time $\tau$ at which the chains meet, and sets $Z_t = Z'_t$ afterward. Then, $ d_{\mbox{TV}}(P_T z, P_T z') \leq \Pr[\tau > T]$. Let $\tau'$ be the (random) time that either $Z_t$ or $Z'_t$ leaves $\mathcal{D}$. 

Then, note that since $L$ is convex inside $\mathcal{D}$ (from Lemma \ref{lem-Conv_L}), we have 
\begin{equation}
    \|Z_t - Z'_t\| \leq \|z-z'\| + 2 dB_t, \forall t \in (0,\tau')
    \label{l:reflcoupling}
\end{equation}  
\Anote{this is exactly the claim in \citejournal{bubeck2018sampling}, Lemma 4}
Let's denote by $\tau''$ the first time a Brownian motion started at 0 hits the value $-\frac{\|z-z'\|}{2}$. Then,  
\begin{align*}
    \Pr[\tau > t] &\leq \Pr[\tau' > t \lor \tau''> t] \\
    &\leq \Pr[\tau' > t]+\Pr[\tau''> t] 
\end{align*}
As in \citejournal{bubeck2018sampling}, we have $\Pr[\tau''> t] \leq \frac{\|z-z'\|}{\sqrt{2 \pi t}}$. On the other hand, by Lemma \ref{lem-concentrationD}, we have $ \Pr[\tau' > t] \leq  \epsilon/4$. This altogether proves \eqref{eq:tvlang}. 

Now, we can finish up as follows. 
Remember that $P$ denotes the stationary distribution of the Langevin chain. We have 
\begin{align*}
   d_{\mbox{TV}}(P_T z, P) &\leq \int_{z' \in \R^d} d_{\mbox{TV}}(P_T z, P_T z') P(z') dz' \\
   &\leq \Pr (z' \notin \mathcal{D}) + \int_{z' \in \mathcal{D}} \frac{\|z-z'\|}{\sqrt{2 \pi T}} P(z') dz' \\ 
   &\leq \epsilon + 2(1-\epsilon) \frac{rad(\mathcal{D})}{\sqrt{2 \pi T}}
\end{align*}
\Dnote{Prolly the expr is $ \epsilon + \frac{\epsilon}{4} (1 - \epsilon) + \frac{rad(\mathcal{D})}{\sqrt{2 \pi T}} (1 - \epsilon)$. }
Since $rad(\D)$ is upper bounded by $\O(1)$ using lemma \ref{def-D}, setting $T = O(1/\epsilon^2)$ we get 
$ d_{\mbox{TV}}(P_T z, P) \leq 2\epsilon$ as we wanted. 
\Dnote{Upto now, we bounded $d_{\mbox{TV}}(P_T z, P)$. But we have already done this in lemma \ref{lem-MainSampling}.}\Anote{agreed}

Proceeding to the discretization part, let us denote by $\hP_T z$ the application of the discretized Langevin diffusion. We have: 
\begin{align*} d_{\mbox{TV}}(\hP_T z, P) &\leq d_{\mbox{TV}}(\hP_T z, P_T z) + d_{\mbox{TV}}(P_T z, P) 
\end{align*} 
Consider the coupling for $\hP_T$ and $P_T$ that uses the same Brownian motion. Same as in \eqref{l:reflcoupling}, if $Z_t, \hZ_t$ are in $\mathcal{D}$, we have 
\begin{equation}
    \|Z_t - \hZ_t\| \leq \|z-z'\| + 2 dB_t +  %\forall t \in (0,\tau') 
    T h L_C \cdot rad(\mathcal{D}) \qquad \forall t \in (0,\tau')
    \label{l:reflcoupling2}
\end{equation}  
where $L_C$ is the Lipschitz constant of $\nabla L$ inside $\mathcal{D}$. 
To see this, consider Lemma 7 in \citejournal{bubeck2018sampling}. We have 
%$$d\|Z_t -Z'_t\|^2_2 = -\langle Z_t - Z'_t, \nabla L(Z_t) - \nabla L(Z'_{\lfloor t/h \rfloor h}\rangle$$  
by Lipschitzness of $L$: 
$$\|\nabla L(\hZ_{\lfloor t/h \rfloor h}) - \nabla L(\hZ_t)\| \leq L_C \|\hZ_{\lfloor t/h \rfloor h} - \hZ_t\|$$ 
%We claim for small enough $h$, 
%$$\langle Z_t - Z'_t, \nabla L(Z_t) - \nabla L(Z'_{\lfloor t/h \rfloor h})\rangle \geq 0$$ 
%which is the same guarantee provided in Lemma 7. 
Then, 
$$\langle Z_t - \hZ_t, \nabla L(Z_t) - \nabla L(\hZ_{\lfloor t/h \rfloor h})\rangle =  \langle Z_t - \hZ_t, \nabla L(Z_t) - \nabla L(\hZ_t)\rangle \pm L_C \|Z_t - \hZ_t\|\|\hZ_{\lfloor t/h \rfloor h} - \hZ_t\|$$  
Using the fact that 
$$\hZ_t = \hZ_{\lfloor t/h \rfloor h} + N(0, (t - \lfloor t/h \rfloor h) I_d) + (t - \lfloor t/h \rfloor h) \nabla L(\hZ_{\lfloor t/h \rfloor h})$$
With high probability \Anote{Add this to the events we are union bounding below when bounding $\Pr[\tau > t]$}, we have 
$\|\hZ_t - \hZ_{\lfloor t/h \rfloor h}\| \leq L_C h \cdot rad(\mathcal{D})$ 

Then, we redo the same analysis of before, with the same notation. We have, for the coupling time $\tau$: 
\begin{align*}
    \Pr[\tau > t] &\leq \Pr[\tau' > t \lor \tau''> t] \\
    &\leq \Pr[\tau' > t]+\Pr[\tau''> t] 
\end{align*}
Again, we have $\Pr[\tau''> t] \leq \frac{\|z-z'\|+ThL_C}{\sqrt{2 \pi T}}$ and by Lemma \ref{lem-concentrationD}, we have $ \Pr[\tau' > t] \leq  \epsilon/4$. 

%We proceed as in Proposition 6 and Lemma 8 in \citejournal{bubeck2018sampling}. Consider the coupling between $\hP_T$ and $P_T$ that uses the same Brownian motion for both. 
