# Supplementary material for: The Effects of Invertibility on the Representational Complexity of Encoders in Variational Autoencoders
Source: arXiv:2107.04652 source file (2021-07-09)
Supplement: Supplementary file 3 [file poincare_constant.tex]

\subsection{Poincar\'e Constant of the Reflected Langevin Diffusion} \label{sS-PCRestricted}

The main lemma of this section will be the following one: 
\begin{lemma} \label{lem-mainpc}
    The Poincar\'e constant of $p(z|x)$ restricted to $\D$ satisfies
    $ \mainpc(\tP) \leq \frac{2}{\pi} rad(\D)$.
\end{lemma}

%The proof is a straightforward calculation, and included in the Appendix. %  \ref{S-lemma_sampling}.  
% ~\ref{AS-perturbation}.
%As a consequence, we can conclude:

%In this section, we prove Lemma \ref{lem-mainpc}. 

First, we prove the convexity of $L(z)$ for $z \in \D$.
(Recall, $\D$ is defined in \ref{lem-concentrationD}.)

\begin{proof}    Using the expression of $\nabla^2 L$ from equation \eqref{eq-nabla2Lz}, we get that
    \begin{equation} \label{eq-nabla2LinD}
        \nabla^2 L(z) \succeq \left( 1 + \frac{1}{\beta^2} \left( m^2 - \left \| \sum_{i \in [d]} \nabla^2 G_i(z) \left( G_i(z) - x_i \right) \right \|_{op} \right) \right) I  
    \end{equation}
    And we have
    \begin{align*}
        \left \| \sum_{i \in [d]} \nabla^2 G_i(z) \left( G_i(z) - x_i \right) \right \|_{op} & \leq \sum_{i \in [d]}  |G_i(z) - x_i| \cdot \left \| \nabla^2 G_i(z) \right \|_{op} \\
        & \leq \sum_{i \in [d]}  |G_i(z) - x_i| \cdot \left \| \nabla^2 G_i(z) \right \|_{op} \\
        & \leq^{(0)} \sqrt{d} \cdot \| G(z) - x \| \cdot \left \| \nabla^2 G(z) \right \|_{op} \\
        & \leq^{(1)} \sqrt{d} \cdot M \|z - \hz\| \cdot \DGtwo  \\
        & \leq \sqrt{d} M \DGtwo \cdot rad(\D) \qquad z \in \D
    \end{align*}
    In $(0)$, we used the fact that $\forall i \in [d], \left\| \nabla^2 G_i(z) \right\|_{op} \leq \| \nabla^2 G(z) \|_{op}$; which can be derived from the $\sup$-definition of the tensor $\ell_2$ norm from \citep{lim2005singular}.
    In $(1)$, we've used Assumption \ref{as-M}.
    Using the expression of $rad(\D)$ from lemma \ref{def-D}, we get
    \begin{align*}
        \left \| \sum_{i \in [d]} \nabla^2 G_i(z) \left( G_i(z) - x_i \right) \right \|_{op} \leq \frac{m^2}{6 \sqrt{d} } \qquad &z \in \D \\
        \leq m^2 \qquad &z \in \D \; \; (\text{since } d \geq 1)
    \end{align*}
    Using this in \eqref{eq-nabla2LinD}, we get $\nabla^2 L(z) \succeq I$ for $z \in \D$.
\end{proof}

Using this, we can prove the bound on the $\mainpc(\tP)$ as below.
\begin{proof}[Proof of Lemma \ref{lem-mainpc}]
   Follows by applying Lemmas  \ref{lem-bebendorf} and \ref{lem-Conv_L}. %for $S \equiv \D$ and $g \equiv L$. %convexity of $L$ in $\D$ is from Lemma \ref{lem-Conv_L}.
\end{proof}
